# Supplementary material for: Relation-aware Meta-learning for Market Segment Demand Prediction with Limited Records
Source: arXiv:2008.00181 source file (2021-01-14)
Supplement: Supplementary file 1 [file appendix.tex]

\appendix
\section{Meta-Testing Algorithm}
\label{sec:app_metatesting}
\begin{algorithm}[h]
    \caption{Meta-Testing Process of RMLDP}
    \label{alg:RMLDP_testing}
    \begin{algorithmic}[1]
    \REQUIRE learned initialization $\theta_0^{*}$; learning rate for gradient update of each segment: $\alpha$; $|\mathcal{T}_c|$: length of sequence in MPFN; Constructed the market segment knowledge graph $\mathcal{G}$; training dataset of segment $s_t$: \begin{small}$\mathcal{D}_t^{tr}$\end{small}; testing dataset of segment $s_t$: \begin{small}$\mathcal{D}_t^{te}$\end{small}
    \STATE Calculate the data-driven segment representation $\mathbf{q}_t^d$ by Eqn.~\eqref{eq:segment_repr} and segment knowledge graph representation $\mathbf{q}_t^g$
    \STATE Concatenate the representations $\mathbf{q}_t^d$ and $\mathbf{q}_t^g$ as $\mathbf{q}_t$
    \STATE Customize the learned model parameter initializations $\theta_{0}^{*}$ by using $\mathbf{q}_t$ and get the customized initialzations $\theta_{0t}^{*}$
    \STATE Update parameters as: $\theta_{t}=\theta^{*}_{0t}-\alpha\nabla_{\theta}\mathcal{L}(\mathcal{D}_t^{tr};\theta)$
    \STATE Evaluate and report the performance on $\mathcal{D}_{t}^{te}$ using optimized parameters $\theta_{t}$
    \end{algorithmic}
\end{algorithm}
